# Supplementary material for: London dispersion forces without density distortion: a path to first principles inclusion in density functional theory
Source: arXiv:2005.05900 source file (2020-05-15)
Supplement: Supplementary file 1 [file si.pdf]

# Supplementary Information: Derivation of the functional derivative

D.P. Kooi, P. Gori-Giorgi

We wish to include our dispersion energy in a self-consistent framework. For this we need the functional derivative of the dispersion energy w.r.t. the densities $\rho^A$, $\rho^B$. We work by implicit differentiation in the basis of the original "atomic" dispersals $\tilde{b}_i(\mathbf{r})$. Our final $b_i(\mathbf{r})$ are related to the "atomic" dispersals $\tilde{b}_i(\mathbf{r})$ by a transformation,

$$b_p(\mathbf{r}) = \sum_i B_{ip}\tilde{b}_i(\mathbf{r}), \tag{1}$$

where the matrix $B$ is obtained from solving the generalized eigenvalue problem,

$$\sum_j \tilde{\tau}_{kj} B_{ji} = \tau_i \sum_j \tilde{S}_{kj} B_{ji} \;\forall\, i, k, \tag{2}$$

where the matrices $\tilde{\tau}$ and $\tilde{S}$ are the matrices of equations 24 b-c in the article, expressed in the "atomic" dispersal basis. In the final expression of the energy, there is a dependence on the eigenvalues $\tau_i$ in the denominator, as well as a dependence on the eigenvectors $\vec{B}_i$ in the numerator via $w_{pq}$, since,

$$w_{pq} = \sum_{ij} B^A_{ip}\tilde{w}_{ij}B^B_{jq}, \tag{3}$$

where again the matrix $\tilde{w}$ is that of equation 24a of the article expressed in the "atomic" dispersal basis. We obtain the derivatives of the eigenvalues and eigenvectors via the usual implicit differentiation. For the eigenvalues and eigenvectors, respectively, we obtain the standard expressions,

$$\frac{\delta\tau_p}{\delta\rho(\mathbf{r})} = \sum_{ij} B_{ip}\frac{\delta\tilde{\tau}_{ij}}{\delta\rho(\mathbf{r})}B_{jp} - \tau_p\sum_{ij} B_{ip}\frac{\delta\tilde{S}_{ij}}{\delta\rho(\mathbf{r})}B_{jp}, \tag{4}$$

$$\frac{\delta B_{ip}}{\delta\rho(\mathbf{r})} = -\frac{1}{2}B_{ip}\sum_{jk} B_{jp}\frac{\delta\tilde{S}_{jk}}{\delta\rho(\mathbf{r})}B_{kp} + \sum_{r\neq p,jk}\frac{1}{\tau_p-\tau_r}\left(B_{jr}\frac{\delta\tilde{\tau}_{jk}}{\delta\rho(\mathbf{r})}B_{kp} - \tau_p B_{jr}\frac{\delta\tilde{S}_{jk}}{\delta\rho(\mathbf{r})}B_{kp}\right)B_{ir}. \tag{5}$$

Care must be taken with the factor $\frac{1}{(\tau_p-\tau_r)}$, since it will diverge in the case of true degeneracy (e.g. when working in spherical symmetry) and will be numerically unstable in the case of near degeneracy. However, in the final expressions we manage to remove these contributions. The functional derivatives of $\tilde{\tau}$, $\tilde{S}$ and $\tilde{w}$ are given by,

$$\frac{\delta\tilde{\tau}_{ij}}{\delta\rho(\mathbf{r})} = \nabla\tilde{b}_i(\mathbf{r})\cdot\nabla\tilde{b}_j(\mathbf{r}), \tag{6}$$

$$\frac{\delta\tilde{S}_{ij}}{\delta\rho(\mathbf{r})} = \tilde{b}_i(\mathbf{r})\left(\tilde{b}_j(\mathbf{r}) + \int d\mathbf{r}' h_{xc}(\mathbf{r},\mathbf{r}')\tilde{b}_j(\mathbf{r}')\right) + \int d\mathbf{r}'\rho(\mathbf{r}')\tilde{b}_i(\mathbf{r}')\int d\mathbf{r}''\frac{\delta h_{xc}(\mathbf{r}',\mathbf{r}'')}{\delta\rho(\mathbf{r})}\tilde{b}_j(\mathbf{r}''), \tag{7}$$

$$\begin{aligned}\frac{\delta\tilde{w}_{ij}}{\delta\rho^A(\mathbf{r})} = &\int d\mathbf{r}_{1_B} w_{\text{disp}}(\mathbf{r},\mathbf{r}_{1_B})\rho^B(\mathbf{r}_{1_B})\left(\tilde{b}^A_i(\mathbf{r}) + \int d\mathbf{r}_{2_A} h^A_{xc}(\mathbf{r},\mathbf{r}_{2_A})\tilde{b}^A_i(\mathbf{r}_{2_A})\right)\\ &\left(\tilde{b}^B_j(\mathbf{r}_{1_B}) + \int d\mathbf{r}_{2_B} h^B_{xc}(\mathbf{r}_{1_B},\mathbf{r}_{2_B})\tilde{b}^B_j(\mathbf{r}_{2_B})\right)\\ &+\int d\mathbf{r}_{1_A}d\mathbf{r}_{1_B} w_{\text{disp}}(\mathbf{r}_{1_A},\mathbf{r}_{1_B})\rho^A(\mathbf{r}_{1_A})\rho^B(\mathbf{r}_{1_B})\int d\mathbf{r}_{2_A}\frac{\delta h^A_{xc}(\mathbf{r}_{1_A},\mathbf{r}_{2_A})}{\delta\rho^A(\mathbf{r})}\tilde{b}^A_i(\mathbf{r}_{2_A})\\ &\left(\tilde{b}^B_j(\mathbf{r}_{1_B}) + \int d\mathbf{r}_{2_B} h^B_{xc}(\mathbf{r}_{1_B},\mathbf{r}_{2_B})\tilde{b}^B_j(\mathbf{r}_{2_B})\right).\end{aligned} \tag{8}$$

The functional derivatives of $\tilde{S}_{ij}$ and $\tilde{w}_{ij}$ can be rewritten in terms of the xc-hole projected dispersals (see main article) and can be further simplified by introducing the exchange-correlation pair function $g_{xc}(\mathbf{r},\mathbf{r}')$, such that $h_{xc}(\mathbf{r},\mathbf{r}') = \rho(\mathbf{r}')g_{xc}(\mathbf{r},\mathbf{r}')$. The functional derivative of $S_{ij}$, for example, becomes

$$\frac{\delta\tilde{S}_{ij}}{\delta\rho(\mathbf{r})} = \tilde{b}_i(\mathbf{r})\tilde{b}_j(\mathbf{r}) - \tilde{b}_{i,xc}(\mathbf{r})\tilde{b}_j(\mathbf{r}) - \tilde{b}_i(\mathbf{r})\tilde{b}_{j,xc}(\mathbf{r}) + g_{ij}^{\text{resp}}(\mathbf{r}), \tag{9}$$

where

$$g_{ij}^{\text{resp}}(\mathbf{r}) = \int d\mathbf{r}' \int d\mathbf{r}'' \rho(\mathbf{r}')\rho(\mathbf{r}'')\tilde{b}_i(\mathbf{r}')\tilde{b}_j(\mathbf{r}'')\frac{\delta g_{xc}(\mathbf{r}',\mathbf{r}'')}{\delta\rho(\mathbf{r})}. \tag{10}$$

The functional derivative of $\tilde{w}_{ij}$ has an analogous but less transparent expression (not reported), where the $A$-xc-hole projected interaction (or $B$ for the other functional derivative) enters, together with the matrix element of the functional derivative of $g_{xc}$ between the interaction and the given dispersal.
We now define the matrices that appear in the main article,

$$\dot{\tau}^A_{pq}(\mathbf{r}) = \sum_{ij} B^A_{ip}\frac{\delta\tilde{\tau}^A_{ij}}{\delta\rho^A(\mathbf{r})}B^A_{jq}, \tag{11}$$

$$\dot{S}^A_{pq}(\mathbf{r}) = \sum_{ij} B^A_{ip}\frac{\delta\tilde{S}^A_{ij}}{\delta\rho^A(\mathbf{r})}B^A_{jq}, \tag{12}$$

$$\dot{w}^A_{pq}(\mathbf{r}) = \sum_{ij} B^A_{ip}\frac{\delta\tilde{w}_{ij}}{\delta\rho^A(\mathbf{r})}B^B_{jq}, \tag{13}$$

and introduce them into the expressions for the derivatives of the eigenvalues and eigenvectors, respectively,

$$\frac{\delta\tau^A_p}{\delta\rho^A(\mathbf{r})} = \dot{\tau}^A_{pp}(\mathbf{r}) - \tau_p\dot{S}^A_{pp}(\mathbf{r}), \tag{14}$$

$$\frac{\delta B_{ip}}{\delta\rho(\mathbf{r})} = -\frac{1}{2}B^A_{ip}\dot{S}^A_{pp}(\mathbf{r}) + \sum_{r\neq p} B_{ir}\frac{1}{\tau_p-\tau_r}\left(\dot{\tau}^A_{rp}(\mathbf{r}) - \tau_p\dot{S}^A_{rp}(\mathbf{r})\right). \tag{15}$$

Now we have all the ingredients necessary to obtain the functional derivative of the final energy of equation 27 of the article, which is repeated here for clarity,

$$E_{\text{disp}}[\rho^A,\rho^B] = -2\sum_{pq}\frac{w^2_{pq}}{\tau^A_p+\tau^B_q}. \tag{16}$$

We take the functional derivative w.r.t. $\rho^A(\mathbf{r})$ and obtain,

$$\frac{\delta E_{\text{disp}}[\rho^A,\rho^B]}{\delta\rho^A(\mathbf{r})} = -4\sum_{pq}\frac{\delta w_{pq}}{\delta\rho^A(\mathbf{r})}\frac{w_{pq}}{\tau^A_p+\tau^B_q} + 2\sum_{pq}\frac{\delta\tau^A_p}{\delta\rho^A(\mathbf{r})}\frac{w^2_{pq}}{(\tau^A_p+\tau^B_q)^2}. \tag{17}$$

To work out the first term, note that,

$$\frac{\delta w_{pq}}{\delta\rho^A(\mathbf{r})} = \sum_{ij}\frac{\delta B^A_{ip}}{\delta\rho^A(\mathbf{r})}\tilde{w}_{ij}B^B_{jq} + \sum_{ij}B^A_{ip}\frac{\delta\tilde{w}_{ij}}{\delta\rho^A(\mathbf{r})}B^B_{jq} = \sum_{ij}\frac{\delta B^A_{ip}}{\delta\rho^A(\mathbf{r})}\tilde{w}_{ij}B^B_{jq} + \dot{w}^A_{pq}(\mathbf{r}). \tag{18}$$

Plugging in the expression for the derivative of the eigenvector,

$$\frac{\delta w_{pq}}{\delta\rho^A(\mathbf{r})} = -\frac{1}{2}\sum_{ij}B^A_{ip}\dot{S}^A_{pp}(\mathbf{r})\tilde{w}_{ij}B^B_{jq} + \sum_{ij}\sum_{r\neq p}\frac{1}{\tau_p-\tau_r}\left(\dot{\tau}^A_{rp}(\mathbf{r}) - \tau_p\dot{S}^A_{rp}(\mathbf{r})\right)B_{ir}\tilde{w}_{ij}B^B_{jq} + \dot{w}^A_{pq}(\mathbf{r}), \tag{19}$$

which can be simplified to,

$$\frac{\delta w_{pq}}{\delta\rho^A(\mathbf{r})} = -\frac{1}{2}\dot{S}^A_{pp}(\mathbf{r})w_{pq} + \sum_{r\neq p}\frac{1}{\tau_p-\tau_r}\left(\dot{\tau}^A_{rp}(\mathbf{r}) - \tau_p\dot{S}^A_{rp}(\mathbf{r})\right)w_{rq} + \dot{w}^A_{pq}(\mathbf{r}). \tag{20}$$

Then we collect all terms of the full functional derivative,

$$\frac{\delta E_{\rm disp}[\rho^A,\rho^B]}{\delta\rho^A(\mathbf{r})} = \sum_{pq}\Bigg(2\left(\dot{\tau}^A_{pp}(\mathbf{r})-\tau^A_p\dot{S}^A_{pp}\right)\frac{w_{pq}}{\tau^A_p+\tau^B_q}+2w_{pq}\dot{S}^A_{pp} \\ -4\sum_{r\neq p}\frac{1}{\tau^A_p-\tau^A_r}\left(\dot{\tau}^A_{rp}(\mathbf{r})-\tau^A_p\dot{S}^A_{rp}(\mathbf{r})\right)w_{rq}-4\dot{w}^A_{pq}(\mathbf{r})\Bigg)\frac{w_{pq}}{\tau^A_p+\tau^B_q}. \tag{21}$$

We would like to combine the terms in such a way to remove the divergent terms $\frac{1}{\tau^A_p-\tau^A_r}$. We do this separately for the terms depending on $\dot{\tau}^A(\mathbf{r})$ and $\dot{S}^A(\mathbf{r})$. First we treat the terms involving $\dot{\tau}^A_{pq}(\mathbf{r})$. We multiply and divide the divergent term by $(\tau^A_r+\tau^B_q)$.

$$2\sum_{pq}\dot{\tau}^A_{pp}(\mathbf{r})\frac{w_{pq}^2}{(\tau^A_p+\tau^B_q)^2}-4\sum_{p\neq r,q}\dot{\tau}^A_{rp}(\mathbf{r})\frac{w_{pq}w_{rq}\tau^A_r}{(\tau^A_p+\tau^B_q)(\tau^A_p-\tau^A_r)(\tau^A_r+\tau^B_q)}-4\sum_{p\neq r,q}\dot{\tau}^A_{rp}(\mathbf{r})\frac{w_{pq}w_{rq}\tau^B_q}{(\tau^A_p+\tau^B_q)(\tau^A_p-\tau^A_r)(\tau^A_r+\tau^B_q)} \tag{22}$$

The denominator of the third (divergent) term is antisymmetric under exchange of $r$ and $p$, while the product $w_{pq}w_{rq}\tau^B_q$ is symmetric, resulting in zero after summation. Now we split the (second) divergent term in half and relabel $r\leftrightarrow p$ in one of the resulting terms, swap $r$ and $p$ in the denominator and combine them to obtain,

$$2\sum_{pq}\dot{\tau}^A_{pp}(\mathbf{r})\frac{w_{pq}^2}{(\tau^A_p+\tau^B_q)^2}-2\sum_{p\neq r,q}\dot{\tau}^A_{rp}(\mathbf{r})\frac{w_{pq}w_{rq}(\tau^A_r-\tau^A_p)}{(\tau^A_p+\tau^B_q)(\tau^A_p-\tau^A_r)(\tau^A_r+\tau^B_q)}. \tag{23}$$

Cancelling the denominator and numerator, one obtains,

$$2\sum_{pq}\dot{\tau}^A_{pp}(\mathbf{r})\frac{w_{pq}^2}{(\tau^A_p+\tau^B_q)^2}+2\sum_{p\neq r,q}\dot{\tau}^A_{rp}(\mathbf{r})\frac{w_{pq}w_{rq}}{(\tau^A_p+\tau^B_q)(\tau^A_r+\tau^B_q)}=2\sum_{pqr}\dot{\tau}^A_{rp}(\mathbf{r})\frac{w_{pq}w_{rq}}{(\tau^A_p+\tau^B_q)(\tau^A_r+\tau^B_q)}. \tag{24}$$

We proceed with the terms involving $\dot{S}^A(\mathbf{r})$,

$$-2\sum_{pq}\dot{S}^A_{pp}(\mathbf{r})\frac{\tau^A_p w_{pq}^2}{(\tau^A_p+\tau^B_q)^2}+2\sum_{pq}\dot{S}^A_{pp}(\mathbf{r})\frac{w_{pq}^2}{\tau^A_p+\tau^B_q}+4\sum_{p\neq r,q}\dot{S}^A_{rp}(\mathbf{r})\frac{\tau^A_p w_{pq}w_{rq}}{(\tau^A_p+\tau^B_q)(\tau^A_p-\tau^A_r)}. \tag{25}$$

First we multiply and divide the second term by $(\tau^A_p+\tau^B_q)$,

$$-2\sum_{pq}\dot{S}^A_{pp}(\mathbf{r})\frac{\tau^A_p w_{pq}^2}{(\tau^A_p+\tau^B_q)^2}+2\sum_{pq}\dot{S}^A_{pp}(\mathbf{r})\frac{w_{pq}^2(\tau^A_p+\tau^B_q)}{(\tau^A_p+\tau^B_q)^2}+4\sum_{p\neq r,q}\dot{S}^A_{rp}(\mathbf{r})\frac{\tau^A_p w_{pq}w_{rq}}{(\tau^A_p+\tau^B_q)(\tau^A_p-\tau^A_r)}, \tag{26}$$

after which the first term is cancelled with the second,

$$2\sum_{pq}\dot{S}^A_{pp}(\mathbf{r})\frac{w_{pq}^2\tau^B_q}{(\tau^A_p+\tau^B_q)^2}+4\sum_{p\neq r,q}\dot{S}^A_{rp}(\mathbf{r})\frac{\tau^A_p w_{pq}w_{rq}}{(\tau^A_p+\tau^B_q)(\tau^A_p-\tau^A_r)}. \tag{27}$$

Now we multiply and divide the divergent term with $(\tau^A_r+\tau^B_q)$, and obtain,

$$2\sum_{pq}\dot{S}^A_{pp}(\mathbf{r})\frac{\tau^B_q w_{pq}^2}{(\tau^A_p+\tau^B_q)^2}+4\sum_{p\neq r,q}\dot{S}^A_{rp}(\mathbf{r})\frac{\tau^A_p\tau^A_r w_{pq}w_{rq}}{(\tau^A_p+\tau^B_q)(\tau^A_p-\tau^A_r)(\tau^A_r+\tau^B_q)}+4\sum_{p\neq r,q}\dot{S}^A_{rp}(\mathbf{r})\frac{\tau^A_p\tau^B_q w_{pq}w_{rq}}{(\tau^A_p+\tau^B_q)(\tau^A_p-\tau^A_r)(\tau^A_r+\tau^B_q)}. \tag{28}$$

By symmetry the second term is zero and we are left with,

$$2\sum_{pq}\dot{S}^A_{pp}(\mathbf{r})\frac{\tau^B_q w_{pq}^2}{(\tau^A_p+\tau^B_q)^2}+4\sum_{p\neq r,q}\dot{S}^A_{rp}(\mathbf{r})\frac{\tau^A_p\tau^B_q w_{pq}w_{rq}}{(\tau^A_p+\tau^B_q)(\tau^A_p-\tau^A_r)(\tau^A_r+\tau^B_q)}. \tag{29}$$

We split the second term in half and relabel $r \leftrightarrow p$ in one of the resulting terms, swap $r$ and $p$ in the denominator and combine them to obtain,

$$2\sum_{pq} \dot{S}^A_{pp}(\mathbf{r}) \frac{\tau^B_q w^2_{pq}}{(\tau^A_p + \tau^B_q)^2} + 2\sum_{p\neq r,q} \dot{S}^A_{rp}(\mathbf{r}) \frac{(\tau^A_p - \tau^A_r)\tau^B_q w_{pq} w_{rq}}{(\tau^A_p + \tau^B_q)(\tau^A_p - \tau^A_r)(\tau^A_r + \tau^B_q)} = 2\sum_{pqr} \dot{S}^A_{rp}(\mathbf{r}) \frac{\tau^B_q w_{pq} w_{rq}}{(\tau^A_p + \tau^B_q)(\tau^A_r + \tau^B_q)}, \tag{30}$$

where we cancelled $(\tau^A_p - \tau^A_r)$ in the numerator and denominator and combined the sums. The final functional derivative is then the one reported in the main article,

$$\frac{\delta E_{\mathrm{disp}}[\rho^A, \rho^B]}{\delta \rho^A(\mathbf{r})} = 2\sum_{pq} \frac{w_{pq}}{\tau^A_p + \tau^B_q} \left( \sum_r \left( \dot{\tau}^A_{rp}(\mathbf{r}) + \tau^B_q \dot{S}^A_{rp}(\mathbf{r}) \right) \frac{w_{rq}}{\tau^A_r + \tau^B_q} - 2\dot{w}^A_{pq}(\mathbf{r}) \right). \tag{31}$$
